# Supplementary material for: Beyond local reconstruction: Geometry-preserving output alignment for binary LLM quantization
Source: arXiv:2512.21651 source file (2026-11-09)
Supplement: Supplementary file 1 [file appendix.tex]

\section{Appendix}
% \paragraph{THE USE OF LARGE LANGUAGE MODELS
% }
% We used a large language model (ChatGPT) to help with editing this paper. It was only used for simple tasks such as fixing typos, rephrasing sentences for clarity, and improving word choice. All ideas, experiments, and analyses were done by the authors, and the use of LLMs does not affect the reproducibility of our work.
\section{Limitations and Future Work}
Our proposed method primarily focuses on preserving token interaction within individual layers, without explicitly modeling interaction across layers or transformer blocks. While the proposed AMP regularizer effectively mitigates layer-wise attention degradation, extending it to capture inter-layer dependencies and block-level attention preservation remains an important direction for future research. Such extensions may further improve the stability and performance of extreme low-bit quantization for large language models.

\section{Impact Statement}
This paper presents work whose goal is to advance the field of Machine Learning. There are many potential societal consequences of our work, none which we feel must be specifically highlighted here.

\section{Proof of Proposition~\ref{prop:amp_eventual_decrease}}
\label{app:amp_proof}

We first state the regularity assumption used in the proof.

\begin{assumption}
\label{assump:amp_eventual_dominance}
For the layer weight $v$, the regularization objective $\mathcal{L}_{Reg}$ has $\beta_v$-Lipschitz continuous gradient with respect to $v$. As the reconstruction objective becomes progressively optimized, the geometry mismatch $G_{v,t}$ persists and induces a non-negligible regularization signal.
\end{assumption}
Assumption~\ref{assump:amp_eventual_dominance} captures the empirical regime observed in our optimization: During the quantization process, as the loss $\mathcal{L}$ decrease and converge,  according to Section \ref{subsec:Anisotropic_preliminary}, the geometry mismatch will be non-negligible over time.

\begin{proposition}[Restated from Proposition 1]
\label{prop:amp_eventual_decrease_appendix}
Under Assumption~\ref{assump:amp_eventual_dominance},  the AMP update is non-increasing for the regularization objective:
\[
\mathcal{L}_{Reg}(v_{t+1}) \le \mathcal{L}_{Reg}(v_t),
\qquad
v_{t+1}=v_t + D_{v,t}.
\] for sufficiently large $t$.
\end{proposition}

\begin{proof}
Since $\mathcal{L}_{Reg}$ has $\beta_v$-Lipschitz continuous gradient with respect to $v$, the descent lemma gives
\begin{equation}
\label{eq:descent_lemma_appendix}
\mathcal{L}_{Reg}(v_{t+1})
\le
\mathcal{L}_{Reg}(v_t)
+
\langle \nabla_v \mathcal{L}_{Reg}(v_t),\, v_{t+1}-v_t\rangle
+
\frac{\beta_v}{2}\|v_{t+1}-v_t\|_2^2.
\end{equation}
Substituting $G_{v,t} = \nabla_v \mathcal{L}_{Reg}(v_t)$ and $v_{t+1}-v_t = D_{v,t}$ yields
\[
\mathcal{L}_{Reg}(v_{t+1})
\le
\mathcal{L}_{Reg}(v_t)
+
\langle G_{v,t}, D_{v,t}\rangle
+
\frac{\beta_v}{2}\|D_{v,t}\|_2^2.
\]
As the training progress, the magnitude of the parameter update $\|D_{v,t}\|_2$ will gradually become insignificant since the optimization converge. By Assumption~\ref{assump:amp_eventual_dominance}, there exists a constant $\mu_v > 0$ and an iteration index $T$ such that for all $t \ge T$ with $D_{v,t} \neq 0$,
\begin{equation}
\label{eq:eventual_dominance}
-\langle G_{v,t}, D_{v,t}\rangle > \mu_v \|D_{v,t}\|_2.
\end{equation}
Therefore, we have,
\[
\langle G_{v,t}, D_{v,t}\rangle < -\mu_v \|D_{v,t}\|_2,
\]
hence
\[
\mathcal{L}_{Reg}(v_{t+1})
<
\mathcal{L}_{Reg}(v_t)
-
\mu_v \|D_{v,t}\|_2
+
\frac{\beta_v}{2}\|D_{v,t}\|_2^2.
\]
Therefore, whenever
\begin{equation}
\label{eq:condition}
\|D_{v,t}\|_2 < \frac{2\mu_v}{\beta_v}.
\end{equation}
we obtain
\[
-\mu_v \|D_{v,t}\|_2 + \frac{\beta_v}{2}\|D_{v,t}\|_2^2 \le 0,
\]
which implies
\[
\mathcal{L}_{Reg}(v_{t+1}) \le \mathcal{L}_{Reg}(v_t).
\]
 This proves the first claim.

Finally, under the empirical behavior of reconstruction optimization, the closed-form update $\Delta v_t$ shrinks over time until convergence to 0, and therefore the AMP-filtered update $D_{v,t} = M_{v,t}\odot \Delta v_t$ also shrinks. Hence condition~\eqref{eq:condition} is eventually satisfied, which implies that $\mathcal{L}_{Reg}(v_t)$ decreases.
\end{proof}
\section{Derivation of closed-forms}
\label{sec:derivation_closedform}
\paragraph{Derivation for $\alpha_c$ } 
The gradient of the objective w.r.t $\alpha_c$ is:

\begin{equation}
\label{eq:derivation_alpha_c_1}
\begin{aligned}
\frac{\partial \mathcal{L}}{\partial \mathrm{diag}(\alpha_c)}
&= \frac{\partial \mathcal{L}}
        {\partial (X W - \widehat{X} \widehat{W})}
   \frac{\partial (X W - \widehat{X} \widehat{W})}
        {\partial \alpha_c} \\
&= -2 B^{\top} \mathrm{diag}(\alpha_r)\widehat{X}^{\top} \\
&\quad \times (X W - \widehat{X} \widehat{W}) \\
&= -2 B^{\top} \mathrm{diag}(\alpha_r)\widehat{X}^{\top} \\
&\quad \times
(X W - \widehat{X}\mathrm{diag}(\alpha_r)B\mathrm{diag}(\alpha_c))
\end{aligned}
\end{equation}

Setting the diagonal of this gradient to 0, we have:
\begin{equation}
\label{eq:derivation_alpha_c_2}
\begin{aligned}
   &\mathrm{Diag}({B^{\top} \mathrm{diag}(\alpha_r)\widehat{S} \mathrm{diag}(\alpha_r)B}) \odot \alpha_c \\
   & = \mathrm{Diag}(B^{\top} \mathrm{diag}(\alpha_r) S W) \\
   &\implies \alpha_c = \frac{\mathrm{Diag}({B}^{T}\mathrm{diag}(\alpha_r) S W )}{\mathrm{Diag}({B}^{T}\mathrm{diag}(\alpha_r) \widehat{S}\mathrm{diag}(\alpha_r) B )} 
\end{aligned}
\end{equation}

\paragraph{Derivation for $\alpha_r$}
The gradient of the objective w.r.t $\alpha_r$ is:
\begin{equation}
\label{eq:derivation_alpha_r_1}
\begin{aligned}
   \frac{\partial \mathcal{L}}{\partial \mathrm{diag}(\alpha_r)} & = \frac{\partial \mathcal{L}}{\partial (X W - \widehat{X} \widehat{W})} \frac{\partial (X W - \widehat{X} \widehat{W})}{\partial \alpha_r} \\
   &= - 2\widehat{X}^{\top} (X W - \widehat{X} \widehat{W}) \mathrm{diag}(\alpha_c) B^{\top}  \\
   &= - 2\widehat{X}^{\top} (X W - \widehat{X} \mathrm{diag}(\alpha_r)B\mathrm{diag}(\alpha_c)) \mathrm{diag}(\alpha_c) B^{\top} \\
\end{aligned}
\end{equation}
Setting the diagonal of this gradient to 0, we have:
\begin{equation}
\label{eq:derivation_alpha_r_2}
\begin{aligned}
   &\quad\mathrm{Diag}(\widehat{S} \mathrm{diag}(\alpha_r)B \mathrm{diag}(\alpha_c \odot \alpha_c) B^{\top}) \\
   & = \mathrm{Diag}( S W \mathrm{diag}(\alpha_c) B^{\top} ) \\
\end{aligned}
\end{equation}
Let $C=B \mathrm{diag}(\alpha_c \odot \alpha_c) B^{\top}$, then we have:
\begin{equation}
\begin{aligned}
     &\mathrm{Diag}(\widehat{S} \mathrm{diag}(\alpha_r)  C  )  =  \mathrm{Diag}( S W \mathrm{diag}(\alpha_c) B^{\top} ) \\
   & \implies  (\widehat{S} \odot C) \alpha_r   =   \mathrm{Diag}( S W \mathrm{diag}(\alpha_c) B^{\top} ) \\
   %& \implies  (\widehat{S} \odot C) \alpha_r   =   \mathrm{Diag}( S W \mathrm{diag}(\alpha_c) B^{\top} ) \\
   & \implies  \alpha_r   = \big( \widehat{S} \odot C \big)^{-1} 
\, \mathrm{Diag}\!\left( S W \mathrm{diag}(\alpha_c) {B}^{\top} \right)
\end{aligned}
\end{equation}

\paragraph{Derivation for $B$}
Explanding the objective loss $\mathcal{L}(.)$ out we have:

\begin{equation}
\label{eq:derivation_B}
\begin{aligned}
    & \operatorname{Tr}\left[(X W - \widehat{X} \widehat{W})(X W - \widehat{X} \widehat{W})^{T}\right] \\
   &= \operatorname{Tr}\left[\widehat{X}\widehat{W} \widehat{W}^{\top}\widehat{X}^{\top} - 2X W  \widehat{W}^{\top}\widehat{X}^{\top}  + \text{const}\right] \\
   &\propto \operatorname{Tr}\left[\widehat{X}^{\top}\widehat{X}\widehat{W} \widehat{W}^{\top}\right]  - 2 \operatorname{Tr}\left[ \widehat{X}^{\top} X W\widehat{W}^{\top}\right]    \\
   &= \operatorname{Tr}\left[\widehat{S}\widehat{W} \widehat{W}^{\top}\right]  - 2 \operatorname{Tr}\left[ S W \widehat{W}^{\top}\right]    \\
   &= \operatorname{Tr}\left[\mathrm{diag}(\alpha_r)S\mathrm{diag}(\alpha_r)B \mathrm{diag}(\alpha_c \odot \alpha_c)B^{\top}\right]  \\
   & \quad - 2 \operatorname{Tr}\left[\mathrm{diag}(\alpha_c)S W \mathrm{diag}(\alpha_r) B^{\top}\right]   \\
   &= \operatorname{Tr}\left[N B  K  B^{\top}\right]   - 2 \operatorname{Tr}\left[ P  B^{\top}\right]   \\
\end{aligned}
\end{equation}

with $N = \mathrm{diag}(\alpha_r)S\mathrm{diag}(\alpha_r)$, $K = \mathrm{diag}(\alpha_c \odot \alpha_c)$, $P = \mathrm{diag}(\alpha_c)S W \mathrm{diag}(\alpha_r)$. 

We denote $\widetilde{B}_{-i}$ and $\widetilde{N}_{-i}$  respectively as the matrix $B$ and $N$ exclude the row $i$. Similarly, $\widetilde{N}_{i,-j}$ denotes the row i of matrix $N$ excluded the $j$ element. Given a row $i$ of $B$, keeping the other row of $B$ as constant, the loss can be expanded as a function of $B_{i,:}$ as:
% \onecoleq{
\begin{equation}
\label{eq:derivation_B_2}
\begin{aligned}
   \mathcal{L}_{MSE}(X,L)   & \propto \operatorname{Tr}\left[N  B  K B^{\top}\right]   - 2 \operatorname{Tr}\left[ PB^{\top}\right] \\
   & = \sum_{i} (N_{i,:}  B  K B_{i,:}^{\top}   - 2 P_{i,:}B_{i,:}^{\top})  \\
   & = \sum_{i} (N_{i,i}  B_{i,:}  K B_{i,:}^{\top} +  \\
   &\widetilde{N}_{i,-i}  \widetilde{B}_{-i}  K B_{i,:}^{\top}   - 2 P_{i,:}B_{i,:}^{\top})  \\
   &\propto \sum_{i} ( \widetilde{N}_{i,-i}  \widetilde{B}_{-i}  K    - 2 P_{i,:}) B_{i,:}^{\top}  \\
\end{aligned}
\end{equation}
% }
Since $B_{i,:}$ is a binary vector, it has a closed-form solution:

\begin{equation}
\label{eq:derivation_B_3}
\begin{aligned}
   B_{i,:}= \mathrm{sign}(\widetilde{N}_{i,-i}  \widetilde{B}_{-i}  K  -  2 P_{i,:} ) \\
\end{aligned}
\end{equation}

The more compacted form of the whole $B$ using this closed-form for each row can be computed as:
\begin{equation}
\label{eq:derivation_B_4}
\begin{aligned}
   B= \mathrm{sign}( [N - \mathrm{diag}(\mathrm{Diag}(N))] B K  - 2 P).
\end{aligned}
\end{equation}
% with $N_{F} = N - \mathrm{diag}(\mathrm{diagonal}(N))$ is the matrix $N$ setting its diagonal to 0.

\section{Additional results}
\label{subsec:addtional_result}

\subsection{Additional implementation details}

It is widely known that block-level loss are more important than layer-wise loss, due to cross-layer dependency across layers within blocks \citep{li2021brecq}. However, naïvely applying output-driven quantization to all layers within a block does not necessarily guarantee minimization of the block-level loss. To ensure stability, we therefore adopt a conservative design choice and restrict output alignment to only the last fully connected layer of each block, which has a direct and dominant influence on the block loss. The remaining layers within each block are quantized using weight-alignment objective in Eq\ref{eq:reconstruction}.

% \begin{table}[h]
% \centering
% \begin{threeparttable}
% \begin{tabular}{c|c|cc}
%     \toprule
%     \multicolumn{2}{c|}{\multirow{2}{*}{\textbf{Model / Method}}} & \multicolumn{2}{c}{\textbf{PPL} ($\downarrow$)} \\ 
%     \cmidrule(r){3-4}
%     \multicolumn{2}{c|}{} & \textbf{C4} & \textbf{WikiText2} \\
%     \midrule
%     \multirow{2}{*}{\textbf{LLama-2-7B}} 
%       & No AMP & 29.12 & 26.24 \\
%       & AMP    & \textbf{19.25} & \textbf{15.42}  \\
%     \cmidrule(r){1-4}
%     \multirow{2}{*}{\textbf{OPT-6.7B}} 
%       & No AMP & 16.35 & 14.74 \\
%       & AMP    & \textbf{16.22} & \textbf{14.56} \\
%     \bottomrule
% \end{tabular}
% \end{threeparttable}
% \caption{Layer-wise ablation of Attention Matrix Preservation (AMP) for LLaMA-2-7B and OPT-6.7B.}
% \label{tab:ablation_AMP}
% \end{table}

\paragraph{Ablation study for output alignment of different layers.}

To investigate the impact of applying output alignment at different layers, we conduct an ablation study in which our method is applied to individual layers within each block of OPT and LLaMA models. The results are reported in Table \ref{tab:ablation_layers}. We observe that output alignment is most effective and consistent when applied to the final layer of each block for both OPT and LLaMA models. In contrast, uniformly applying output alignment to other layers can lead to degraded performance and may even underperform weight alignment. This behavior is expected, as discussed in Section \ref{subsec:Error_propa_preliminary}, since output alignment at intermediate layers does not guarantee a reduction in block-level loss. These observations suggest a promising future direction: rather than uniformly applying the same optimization strategy to specific layers across blocks, we could adaptively determine, for each block, which layers are better suited for weight alignment and which benefit more from output alignment.

\begin{table}[t]
\centering

\begin{threeparttable}
\begin{tabular}{c|c|cc}
    \toprule
    \multicolumn{2}{c|}{\multirow{2}{*}{\textbf{Model / Layer}}} & \multicolumn{2}{c}{\textbf{PPL} ($\downarrow$)} \\ 
    \cmidrule(r){3-4}
    \multicolumn{2}{c|}{} & \textbf{C4} & \textbf{WikiText2} \\
    \midrule
    \multirow{5}{*}{\textbf{Llama-2-7B}} 
      & Query         & 20.08 & 15.85 \\
      & Key           & 20.80 & 16.75 \\
      & Value         & 21.44 & 17.82 \\
      & Attn Out      & 21.02 & 18.11 \\
      \rowcolor{midgray}& \textbf{Final FC} & \textbf{19.25} & \textbf{15.42} \\
    \cmidrule(r){1-4}
    \multirow{5}{*}{\textbf{OPT-6.7B}} 
      & Query         & 17.15 & 15.15 \\
      & Key           & 17.13 & 15.06 \\
      & Value         & 17.12 & 14.81 \\
      & Attn Out      & 17.05 & 15.55 \\
      \rowcolor{midgray}& \textbf{Final FC} & \textbf{16.22} & \textbf{14.56} \\
    \bottomrule
\end{tabular}
\end{threeparttable}
\caption{Ablation study of applying our method to different layers (Q, K, V, Out, Final) of each block for LLaMA-2-7B and OPT-6.7B, evaluated on C4 and WikiText2.}
\label{tab:ablation_layers}
\end{table}

\paragraph{Ablation study for the size of the calibration set.}
We provide additional ablation study about the effective of our method when the size of the calibration set varies. The results are provided in Table \ref{tab:calibration_size_opt}. The results demonstrates that our method are effective even when the number of calibration samples is small.
\begin{table}[t]
\centering

\begin{tabular}{c|c|cc}
    \toprule
    \multirow{2}{*}{\textbf{Size}} 
    & \multirow{2}{*}{\textbf{Method}} 
    & \multicolumn{2}{c}{\textbf{PPL} $(\downarrow)$} \\ 
    \cmidrule(r){3-4}
     &  & \textbf{C4} & \textbf{WikiText2}  \\
    \midrule
    \multirow{2}{*}{32}  
      & ARB-RC & 22.77 & 22.50 \\
      & Ours   & \textbf{21.25} & \textbf{19.84} \\
    \cmidrule(r){1-4}
    \multirow{2}{*}{128} 
      & ARB-RC & 21.76 & 19.84 \\
      & Ours   & \textbf{19.90} & \textbf{18.25} \\
    \bottomrule
\end{tabular}
\caption{Ablation study on the calibration set size for OPT-2.7B.}
\label{tab:calibration_size_opt}
\end{table}

% -------- Left table (layer ablation) ----------

\paragraph{Additional zero-shot QA results for LLama models.}

We provide additional results of our method using 8 different zero-shot QA datasets, over Llama architectures
\begin{table*}[H]
\centering

\label{tab:LLaMA_eval}
\setlength{\tabcolsep}{7pt} % column padding
 % row height
\resizebox{\linewidth}{!}{
\begin{tabular}{c|c|c|cccccccc>{\columncolor{midgray}}c}
\toprule
\textbf{Model Size} & \textbf{Method} & \textbf{Bits} & 
Boolq & Lambada & Piqa & OPQA & Winogrande & Arc-E & Arc-C & Hellaswag & Avg \\
\midrule
\textbf{LLaMA-2-7B} & ARB-RC & 1.06 & 67.74 & 51.87 & 65.51 & 29.8 & 59.98 & 46.8 & 28.24 & 48.1 & 49.75 \\
 & \textbf{Ours} &1.06 &  66.45  & 52.53 & 68.12 &29.8 & 56.99 & 30.3 & 51.56 & 49.24 &  \textbf{50.62}\\
\midrule

\textbf{LLaMA-2-13B} & ARB-RC & 1.06  & 74.86 & 66.23  & 71.16& 33.0 & 62.04 & 57.37 & 33.36 & 50.46 & 56.06 \\
 & \textbf{Ours} & 1.06 & 72.02 & 68.99 & 72.58 & 36.0 & 63.14 & 59.85 & 33.7 & 53.92 & \textbf{57.53} \\
\midrule
\textbf{LLaMA-3-8B} & ARB-RC & 1.06 & 67.58 & 48.85 & 62.73 & 29.2 & 57.38 & 42.97 & 24.57 & 43.63 & 47.11 \\
 & \textbf{Ours} & 1.06 & 66.54 & 49.35 & 63.33 & 30.4 & 56.2 & 45.66 & 26.02 & 44.21 & \textbf{47.71} \\
\bottomrule
\end{tabular}}
\caption{Evaluation the accuracy $(\uparrow)$ of LLaMA models using ARB-RC and our method over zero-shot QA benchmarks.}
\end{table*}

\paragraph{Ablation study for the hyper-parameter $k$}
We provide additional ablation study for the hyper-parameter $k$ in \cref{tab:ablation_k}. In practice, we adopt $k=5$ for stable performance across architecture.
\begin{table}[H]
\centering
\renewcommand\tabcolsep{6pt}

\begin{tabular}{l|c|cc}
    \toprule[1.2pt]
    \multirow{2}{*}{\textbf{Model}} & \multirow{2}{*}{\textbf{k}} & \multicolumn{2}{c}{\textbf{PPL} $(\downarrow)$} \\ 
    \cmidrule(r){3-4}
     &  & \textbf{C4} & \textbf{WikiText2}  \\
    \midrule
    \multirow{3}{*}{\textbf{OPT-6.7B}} & 1  & 16.24 & 14.67 \\
              & 5 & 16.22 & 14.56 \\
              & 10 & 16.21 & 14.40 \\
    \midrule
    \multirow{3}{*}{\textbf{Llama-2-7B}}  & 1  & 20.16 & 16.26 \\
              & 5 & 19.25 & 15.42 \\
              & 10 & 20.00 & 16.42 \\
    \bottomrule[1.2pt]
\end{tabular}

\caption{Ablation study for the hyper-parameter $k$.}
\label{tab:ablation_k}
\end{table}

\section{Proposed learning algorithm}
\label{app:learning_algorithm}

    \begin{algorithm*}[th]
        \caption{Our-RC}
        \label{alg:our-rc}
        \begin{algorithmic}[1]
            \Procedure{Our-RC}{$W, S, \widehat{S}, T, k$}
                \LComment{$W \in \mathbb{R}^{d_{in}\times d_{out}}$: full-precision weight}
                \LComment{$S \in \mathbb{R}^{d_{in}\times d_{in}}$: Gram matrix $X^{\top} \widehat{X}$}
                \LComment{$\hat{S} \in \mathbb{R}^{d_{in}\times d_{in}}$: Gram matrix  $\widehat{X}^{\top} \widehat{X}$}
                \LComment{$T$: iteration rounds}
                \State Initialize $\widehat{W}, \alpha_r, \alpha_c, B$
                \State Initialize $M \gets S W W^{T} S^{T}$
                \For{iter = 1:$T$}
                    \State \(\alpha^{*}_r \gets\) \Call{refine-$\alpha_{r}$}{$S, \widehat{S}, W, B, \alpha_c, M$}
                    \State \(M^r \gets\) \Call{AMP-$\alpha_r$}{$M, B, \alpha_r, \alpha_c$}
                    \State $\alpha_r \leftarrow \alpha_r * (1 - M^r) + \alpha^{*}_r * M^r$
                    %\STATE $\widehat{W} = \mathrm{diag}(\alpha_r)B\mathrm{diag}(\alpha_c)$
                    \If{ $(\mathrm{iter} + 1) \bmod k == 0$}
                        \State $\alpha^{*}_c \leftarrow \text{refine-}\alpha_c(S,\widehat{S},W,B,\alpha_r)$
                        \State \(M^c \gets\) \Call{AMP-$\alpha_c$}{$M, B, \alpha_r, \alpha_c$}
                        \State $\alpha_c \leftarrow \alpha_c * (1 - M^c) + \alpha^{*}_c * M^c$
                    \EndIf
                    %\STATE $\widehat{W} = \mathrm{diag}(\alpha_r)B\mathrm{diag}(\alpha_c)$
                    \State \(B^{*} \gets\) \Call{refine-B}{$S, \widehat{S}, W, B, \alpha_c$}
                    \State \(M^B, i \gets\) \Call{AMP-B}{$M, B, \alpha_r, \alpha_c$}
                    %\STATE $\widehat{W} = \mathrm{diag}(\alpha_r)B\mathrm{diag}(\alpha_c)$
                    \State $B_{i,:} \leftarrow B_{i,:} * (1 - M^B_{i,:}) + B^{*}_{i,:} *  M^B_{i,:}$

                    \State \(B^{*} \gets\) \Call{refine-B}{$S, \widehat{S}, W, B, \alpha_c$}
                    \State \(M^B, i \gets\) \Call{AMP-B}{$M, B, \alpha_r, \alpha_c$}
                    \State $B_{i,:} \leftarrow B_{i,:} * (1 - M^B_{i,:}) + B^{*}_{i,:} *  M^B_{i,:}$
                \EndFor
                \State \Return $\widehat{W}$
            \EndProcedure
        \end{algorithmic}
    \end{algorithm*}

    \begin{algorithm*}[th]
        \caption{Auxiliary functions}
        \label{algorithm:auxiliary}
        \begin{multicols}{2}
        \begin{algorithmic}[1]
            \Procedure{refine-$\alpha_{r}$}{$S,\widehat{S},W,B,\alpha_c,M$}
                \State $\mathcal{B} = B \, \mathrm{diag}(\alpha_c \odot \alpha_r) \, {B}^{\top}$
                \State $\mathrm{matrix} := \widehat{S} \odot \mathcal{B}$
                \State $\mathrm{target} := S W \mathrm{diag}(\alpha_c) {B}^{\top}$
                \State \(\alpha_r \gets\) \Call{solve}{matrix, target}
                \State \Return $\alpha_r$
            \EndProcedure
            \Statex
            \Procedure{refine-$\alpha_c$}{$S,\widehat{S},W,B,\alpha_r$}
                \State $\mathrm{num} := \mathrm{Diag}({B}^{\top}\mathrm{diag}(\alpha_r) S  W )$
                \State $\mathrm{den} := \mathrm{Diag}({B}^{\top}\mathrm{diag}(\alpha_r) \widehat{S}\mathrm{diag}(\alpha_r) B )$
                \State $\alpha_c := \mathrm{num} / \mathrm{den}$
                \State \Return $\alpha_c$
            \EndProcedure
            \Statex
            \Procedure{refine-B}{$S,\widehat{S},W,\alpha_r,\alpha_c$}
                \State $N = \mathrm{diag}(\alpha_r)S \mathrm{diag}(\alpha_r)$
                \State $K = \mathrm{diag}(\alpha_c \odot \alpha_c)$
                \State $P = \mathrm{diag}(\alpha_c)W^{\top}S \mathrm{diag}(\alpha_r)$
                \State $\mathbf{B} = [N - \mathrm{diag}(\mathrm{Diag}(N))] B K  - 2 P$
                \State $B^{*} = \mathrm{sign}(B )$
                \State $i \gets \operatorname*{argmax}_{j} \sum_{k} \left( B \odot \mathbf{B} \right)_{j,k}$
                \State \Return $B^{*},i$
            \EndProcedure
            \Statex
            \Procedure{AMP\_B}{$M, B, \alpha_r, \alpha_c$}
                \State $\widehat{W} = \mathrm{diag}(\alpha_r)B\mathrm{diag}(\alpha_c)$
                \State $M^B =  \mathrm{sign}(\mathrm{diag}(\alpha_r)M \widehat{W}\mathrm{diag}(\alpha_c))$
                \State \Return $M^B$
            \EndProcedure
            \Statex
            \Procedure{AMP-$\alpha_r$}{$M, B, \alpha_r, \alpha_c$}
                \State $\widehat{W} = \mathrm{diag}(\alpha_r)B\mathrm{diag}(\alpha_c)$
                \State $M^r =  \mathrm{sign}(\mathrm{Diag}(M \widehat{W}\mathrm{diag}(\alpha_c) B^{\top}))$
                \State \Return $M^r$
            \EndProcedure
            \Statex
            \Procedure{AMP-$\alpha_c$}{$M, B, \alpha_r, \alpha_c$}
                \State $\widehat{W} = \mathrm{diag}(\alpha_r)B\mathrm{diag}(\alpha_c)$
                \State $M^c = \mathrm{sign}(\mathrm{Diag}(B^{\top} \mathrm{diag}(\alpha_r)M \widehat{W}))$ 
                \State \Return $M^c$
            \EndProcedure
        \end{algorithmic}
        \end{multicols}
    \end{algorithm*}

\clearpage
